# Supplementary material for: Atomic Decompositions of Periodic Electronic-Structure Simulations
Source: arXiv:2407.10148 ancillary file (2024-09-30)
Supplement: Supplementary file 1 [file si.pdf]

# Supporting Information: Atomic Decompositions of Periodic Electronic-Structure Simulations

Luna Zamok and Janus J. Eriksen*

*DTU Chemistry, Technical University of Denmark*

*Kemitorvet Bldg. 206, 2800 Kgs. Lyngby, Denmark*

E-mail: janus@dtu.dk

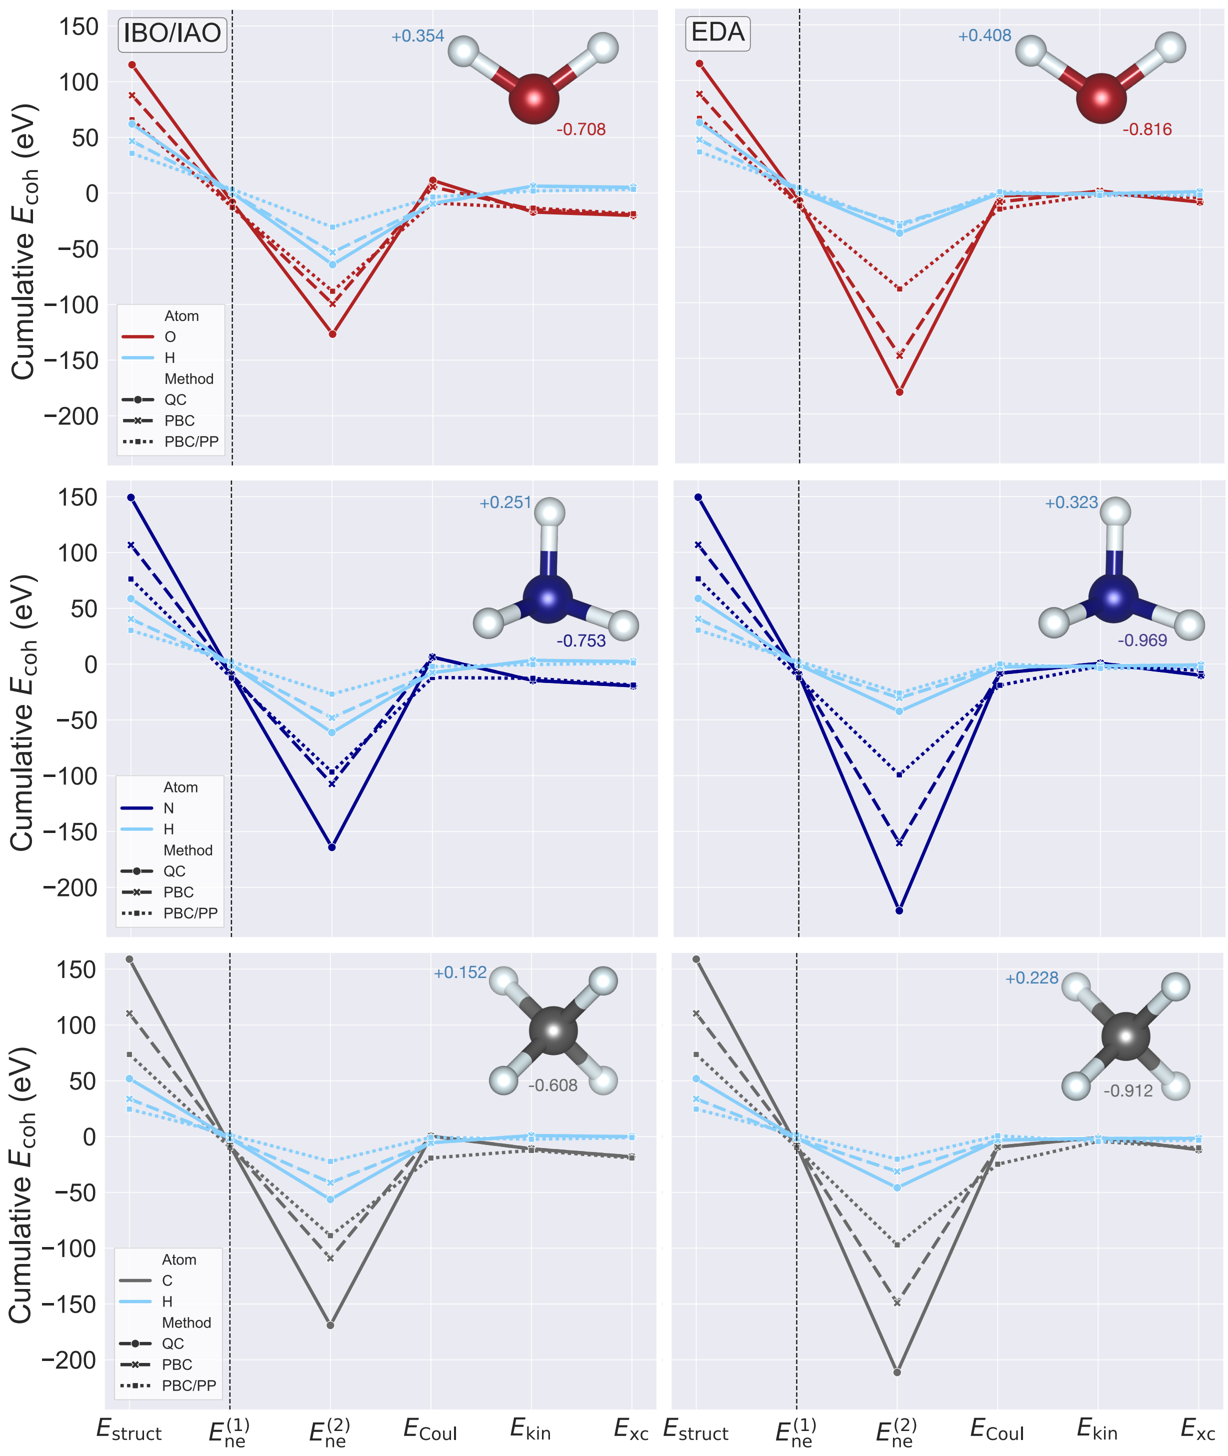


Figure S1: Atomic cohesive energies for $H_2O$, $NH_3$, and $CH_4$, computed via standard quantum-chemical (QC) simulations and employing PBCs, either without or with pseudopotentials and corresponding basis sets (PBC/PP). The insets show IAO-based (left) and standard (right) Mulliken charges derived from the all-electron PBC simulations, and the vertical lines separate contributions to atomic energies common to both decompositions.

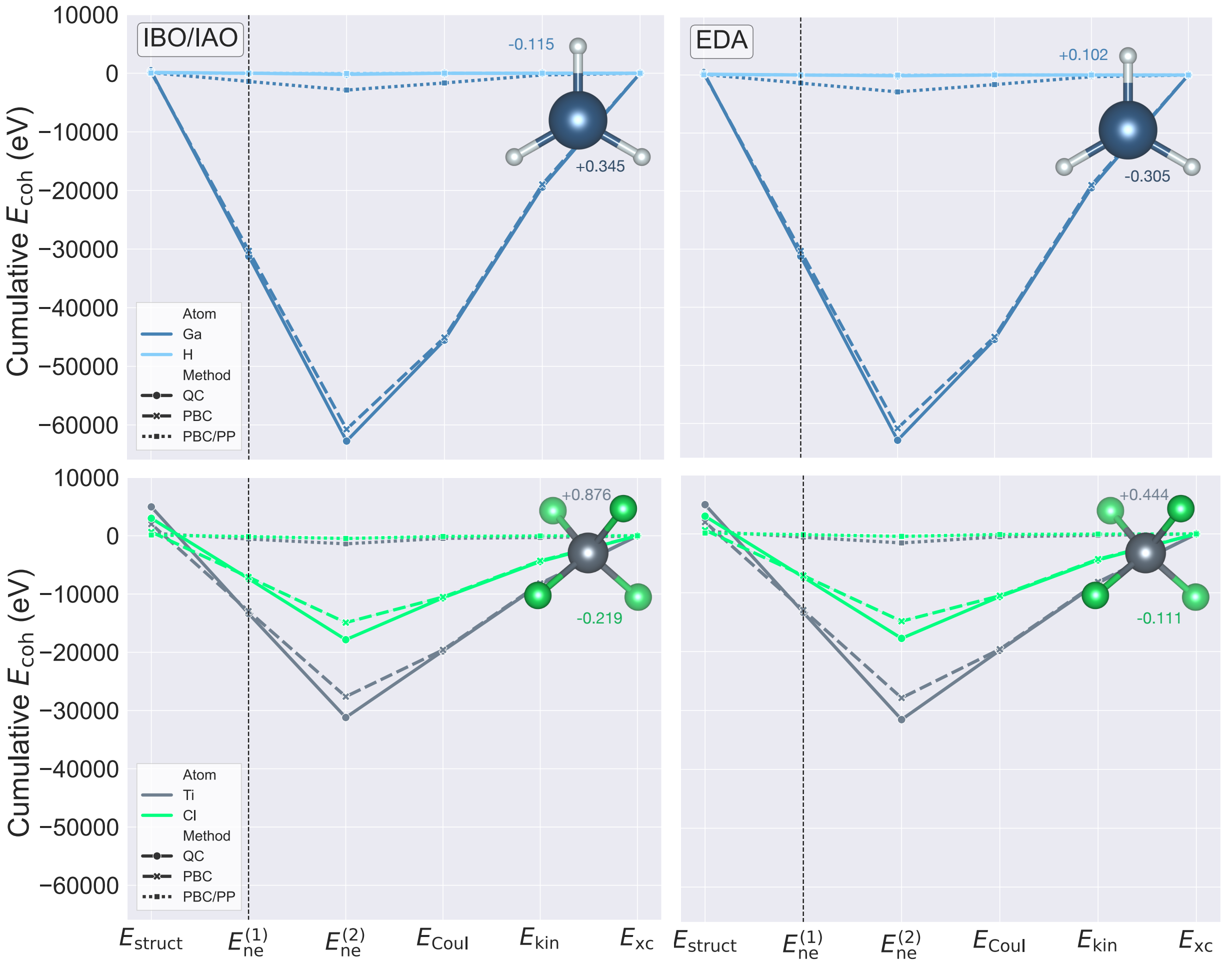


Figure S2: Atomic cohesive energies for $GaH_3$ and $TiCl_4$, cf. Fig. S1 for details.

Table S1: Atomic cohesive energies (in eV) from Fig. 1 of the main study.

| Atom | QC | | PBC | | PBC/PP | |
|---|---|---|---|---|---|---|
| | EDA | IBO/IAO | EDA | IBO/IAO | EDA | IBO/IAO |
| | | | $H_2O$ | | | |
| O | -9.4593 | -20.1458 | -9.4008 | -19.5206 | -5.4823 | -18.5447 |
| H | -0.1223 | 5.2209 | -0.1219 | 4.9380 | -3.1448 | 3.3873 |
| H | -0.1223 | 5.2209 | -0.1219 | 4.9380 | -3.1448 | 3.3873 |
| Total | -9.7040 | -9.7039 | -9.6445 | -9.6445 | -11.7701 | -11.7701 |
| | | | $NH_3$ | | | |
| N | -10.1854 | -19.4982 | -10.1295 | -19.4529 | -5.66402 | -18.7449 |
| H | -0.8333 | 2.2708 | -0.8541 | 2.2534 | -3.3176 | 1.0425 |
| H | -0.8333 | 2.2708 | -0.8541 | 2.2534 | -3.3176 | 1.0425 |
| H | -0.8333 | 2.2708 | -0.8541 | 2.2534 | -3.3176 | 1.0425 |
| Total | -12.6859 | -12.6859 | -12.6926 | -12.6926 | -15.6172 | -15.6172 |
| | | | $CH_4$ | | | |
| C | -11.8100 | -18.1634 | -11.7558 | -18.1177 | -10.1198 | -19.1852 |
| H | -1.6285 | -0.0402 | -1.6424 | -0.0520 | -3.1869 | -0.9205 |
| H | -1.6285 | -0.0402 | -1.6424 | -0.0520 | -3.1869 | -0.9205 |
| H | -1.6285 | -0.0402 | -1.6424 | -0.0520 | -3.1869 | -0.9205 |
| H | -1.6285 | -0.0402 | -1.6424 | -0.0520 | -3.1869 | -0.9205 |
| Total | -18.3241 | -18.3241 | -18.3255 | -18.3255 | -22.8674 | -22.8674 |
| | | | $GaH_3$ | | | |
| Ga | -3.5884 | -4.4323 | -3.5485 | -4.5167 | -3.1471 | 2.4893 |
| H | -1.4889 | -1.2077 | -1.5039 | -1.1811 | -2.6004 | -4.4794 |
| H | -1.4889 | -1.2077 | -1.5039 | -1.1811 | -2.6004 | -4.4794 |
| H | -1.4889 | -1.2077 | -1.5039 | -1.1811 | -2.6004 | -4.4794 |
| Total | -8.0551 | -8.0551 | -8.0601 | -8.0601 | -10.9483 | -10.9483 |
| | | | $TiCl_4$ | | | |
| Ti | -16.7040 | -19.5198 | -9.0491 | -12.2624 | -8.0987 | -49.2529 |
| Cl | -2.6539 | -1.9410 | -2.5837 | -1.7804 | -2.8388 | 7.4499 |
| Cl | -2.6539 | -1.9410 | -2.5837 | -1.7804 | -2.8388 | 7.4499 |
| Cl | -2.6539 | -1.9410 | -2.5837 | -1.7804 | -2.8388 | 7.4499 |
| Cl | -2.6539 | -1.9410 | -2.5837 | -1.7804 | -2.8388 | 7.4499 |
| Total | -27.3195 | -27.3195 | -19.3840 | -19.3840 | -19.4533 | -19.4533 |

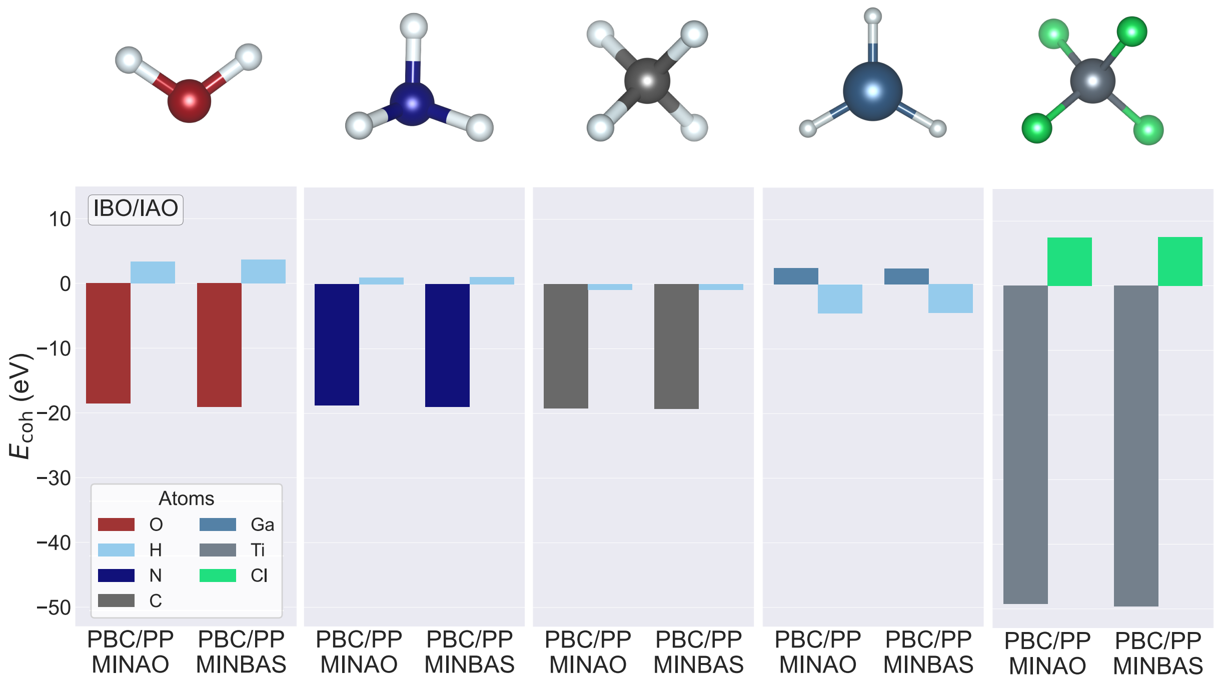


Figure S3: Atomic cohesive energies for $H_2O$, $NH_3$, $CH_4$, $GaH_3$, and $TiCl_4$ computed using PBCs with pseudopotentials (PBC/PP). The minimal basis sets used in calculating IAO charges and constructing IBOs were either MINAO from Ref. S1 or the PP-adapted min-pbe (MINBAS), as distributed with `CP2K` software package.[S2]

Table S2: Partial charges of the atoms in the PAN polymer of Fig. 2 of the main study. The PBC charges have been computed using a grid of 7 $\boldsymbol{k}$-points, and the QC charges have been computed for the central unit of a polymer with 7 repeating units.

| Atom | QC | PBC | PBC/PP |
|---|---|---|---|
| IAO-based Mulliken | | | |
| C1 | −0.130 | −0.132 | −0.125 |
| C2 | −0.230 | −0.238 | −0.229 |
| C3 | +0.104 | +0.105 | +0.098 |
| N | −0.217 | −0.216 | −0.212 |
| H1 | +0.180 | +0.183 | +0.177 |
| H2 | +0.146 | +0.149 | +0.146 |
| Standard Mulliken | | | |
| C1 | −0.148 | −0.049 | +0.004 |
| C2 | −0.466 | −0.180 | +0.042 |
| C3 | −0.058 | −0.077 | −0.512 |
| N | −0.106 | −0.104 | +0.195 |
| H1 | +0.313 | +0.175 | +0.112 |
| H2 | +0.232 | +0.118 | +0.080 |

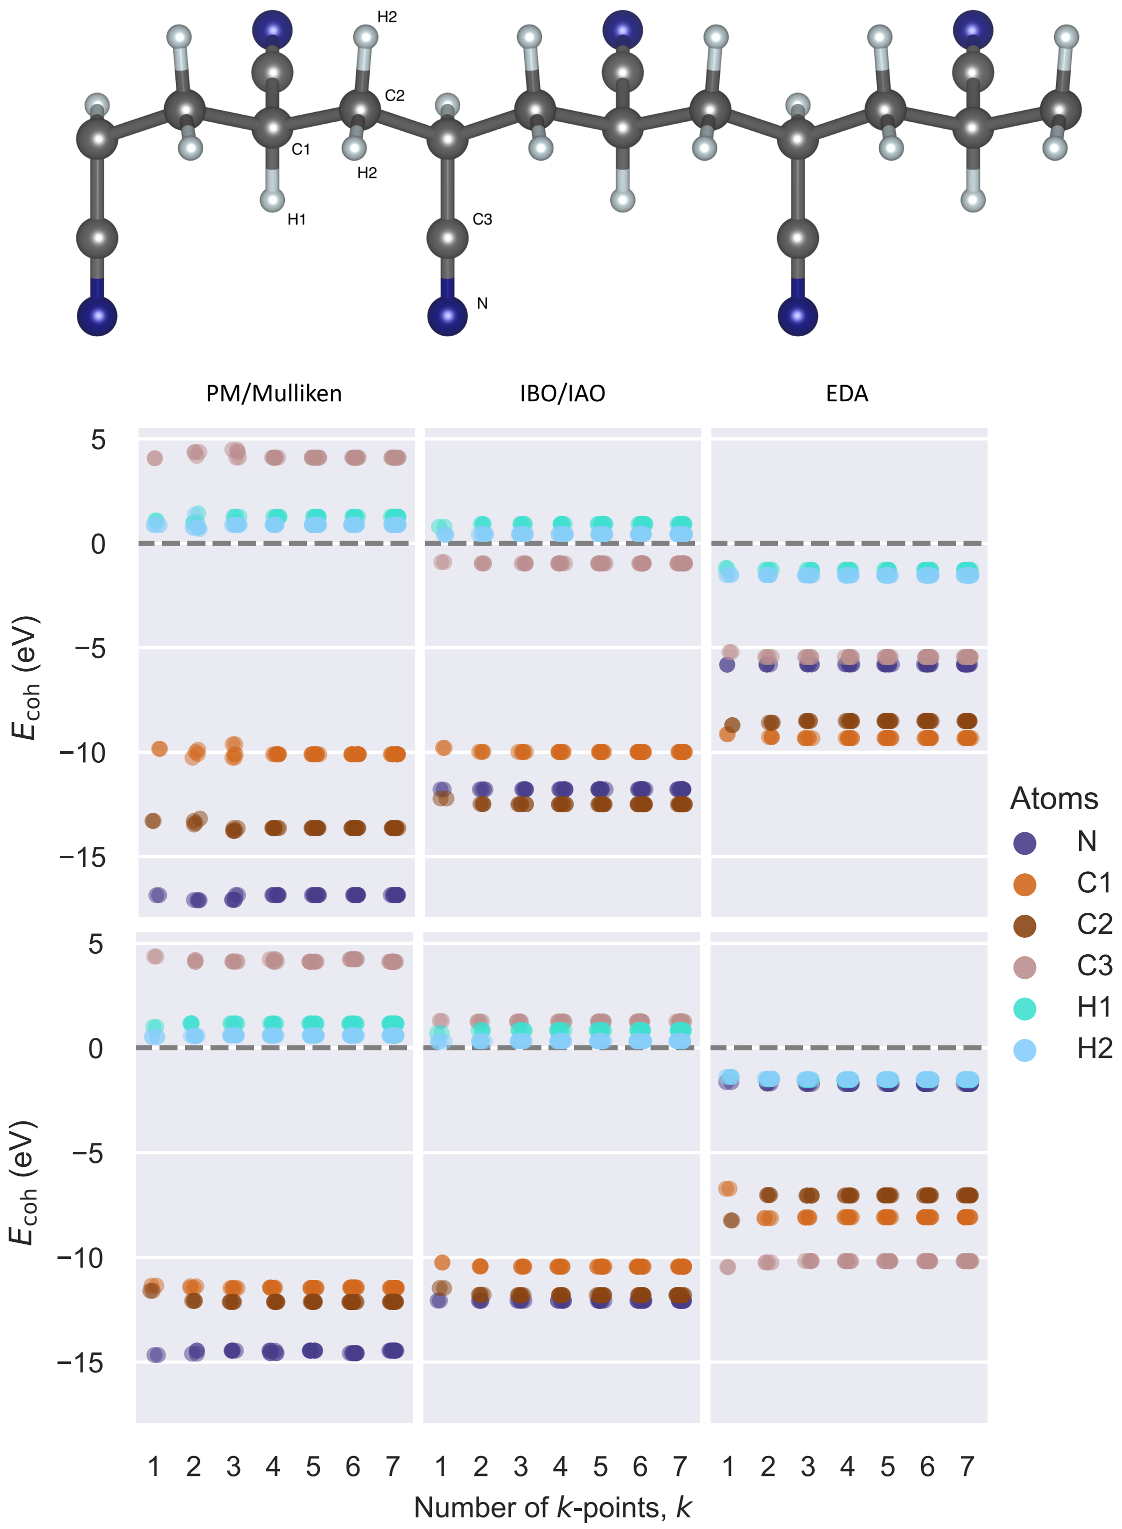


Figure S4: Atomic cohesive energies for the PAN polymer in Fig. 2, computed using PBCs and either all-electron basis sets (upper panel) or pseudopotentials (lower panel).

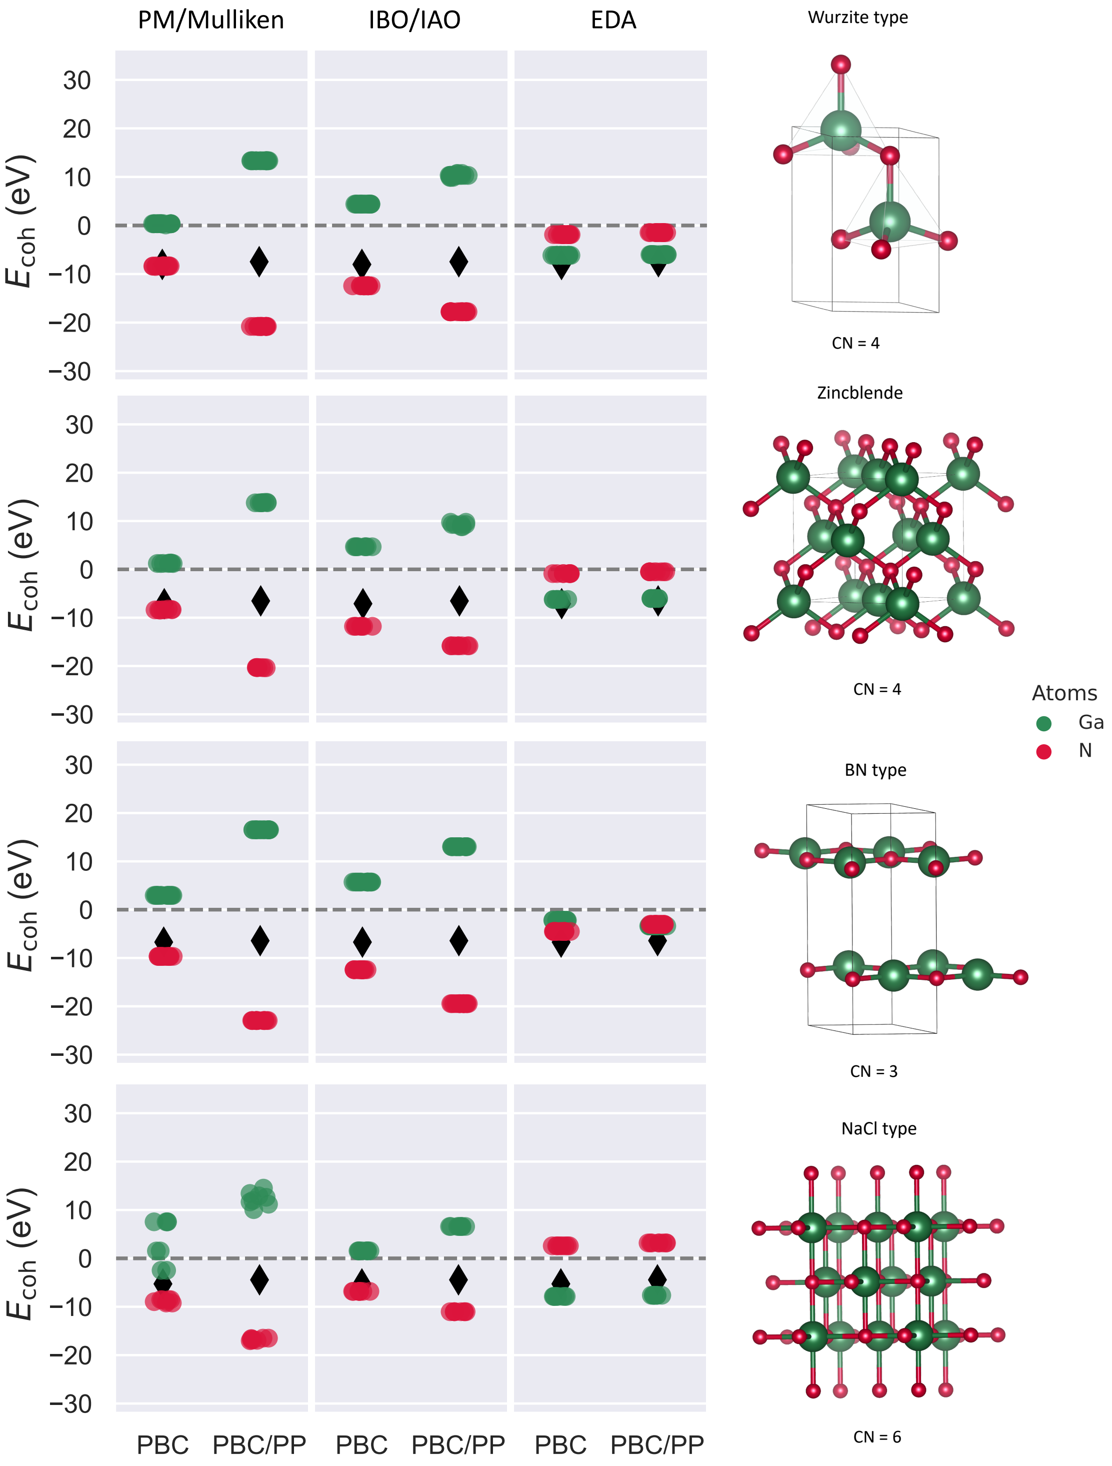


Figure S5: PBC and PBC/PP atomic cohesive energies for different GaN polymorphs, calculated using a grid of $2^3$ $\boldsymbol{k}$-points. Black markers represent total cohesive energies, and the panel on the right shows coordination numbers.

# References


(S1) Knizia, G. Intrinsic Atomic Orbitals: An Unbiased Bridge Between Quantum Theory and Chemical Concepts. J. Chem. Theory Comput. **2013**, 9, 4834.

(S2) Kühne, T. D.; Iannuzzi, M.; Del Ben, M.; Rybkin, V. V.; Seewald, P.; Stein, F.; Laino, T.; Khaliullin, R. Z.; Schütt, O.; Schiffmann, F.; Golze, D.; Wilhelm, J.; Chulkov, S.; Bani-Hashemian, M. H.; Weber, V.; Borštnik, U.; Taillefumier, M.; Jakobovits, A. S.; Lazzaro, A.; Pabst, H.; Müller, T.; Schade, R.; Guidon, M.; Andermatt, S.; Holmberg, N.; Schenter, G. K.; Hehn, A.; Bussy, A.; Belleflamme, F.; Tabacchi, G.; Glöß, A.; Lass, M.; Bethune, I.; Mundy, C. J.; Plessl, C.; Watkins, M.; VandeVondele, J.; Krack, M.; Hutter, J. CP2K: An Electronic Structure and Molecular Dynamics Software Package – Quickstep: Efficient and Accurate Electronic Structure Calculations. J. Chem. Phys. **2020**, 152, 194103.
